# Supplementary material for: Data-Driven Protection Levels for Camera and 3D Map-based Safe Urban Localization
Source: arXiv:2101.06379 source file (2021-04-13)
Supplement: Supplementary file 1 [file appendix.tex]

\section{Appendix}
\label{apdx:rot_cov}
\subsection*{Covariance Matrix for Uncertainty in DNN-based Rotation}
\chl{In this section, we derive an expression for approximating the covariance matrix $\Sigma^{(i)}_t$ for the $i$th position error sample $\Delta\*x^{(i)}_t$ by incorporating the uncertainty in the rotation matrix $\tilde{R}_t$ associated with the DNN-based rotation error $\Delta \tilde{\*r}_t$ for the state estimate $\*s_t$. 

From equation}~\ref{eqn:transform}\chl{, $\Delta\*x^{(i)}_t$ is defined in terms of candidate state position error $\Delta \*x^i_t$, $\tilde{R}_t$, and the known translation offset $\*t^i$}
\begin{equation}
    \cmhl{\Delta\*x^{(i)}_t = \Delta \*x^i_t - \tilde{R}_t^\top\*t^i.}
\end{equation}   
 \chl{The resulting covariance matrix $\Sigma^{(i)}_t$ in terms of the covariance matrix $\Sigma^i_t$ for $\Delta \*x^i_t$, $\tilde{R}_t$ and $\*t^i$ is}
 \begin{equation}
    \cmhl{\Sigma^{(i)}_t = \Sigma^i_t + \textrm{Var}[\tilde{R}_t^\top\*t^i].}
 \end{equation}

\chl{Assuming small errors in determining the true rotation offsets between state estimate $\*s_t$ and the true state $\*s^*_t$, we consider the random variable $R'\tilde{R}_t^\top\*t^i$ where $R'$ represents the random rotation matrix corresponding to small angular deviations}~\cite{barfoot_pose_2011}\chl{. Using $R'\tilde{R}_t^\top\*t^i$, we approximate the covariance matrix $\Sigma^{(i)}_t$ as}
\begin{align*}
	\cmhl{\Sigma^{(i)}_t} &\cmhl{\approx \Sigma^i_t + \textrm{Var}[R'\tilde{R}_t^\top\*t^i]}
    \\
    & \cmhl{\approx \Sigma^i_t + \E[(R'-I)(\tilde{R}_t^\top\*t^i)(\tilde{R}_t^\top\*t^i)^\top(R'-I)^\top]}
    \\
	\cmhl{[ \Sigma^{(i)}_t]_{i'j'}} 
    &\cmhl{ = [ \Sigma^i_t ]_{i'j'} + \E[(\*r'_{i'})^\top (\tilde{R}_t^\top\*t^i)(\tilde{R}_t^\top\*t^i)^\top (\*r'_{j'})]}
    \\
    &\cmhl{ = [ \Sigma^i_t ]_{i'j'} + \mathrm{Tr}\left((\tilde{R}_t^\top\*t^i)(\tilde{R}_t^\top\*t^i)^\top \E[(\*r'_{i'})(\*r'_{j'})^\top] \right)}
    \\
    &\cmhl{ = [ \Sigma^i_t ]_{i'j'} + \mathrm{Tr}\left((\tilde{R}_t^\top\*t^i)(\tilde{R}_t^\top\*t^i)^\top Q_{i'j'} \right),} \numberthis
\end{align*}
\chl{where $(\*r'_{i})^\top$ represents the $i$th row vector in $R'-I$. Since errors in $\tilde{R}$ depend on the DNN output, we specify $R'$ through the empirical distribution of the angular deviations in $\tilde{R}$ as observed on the training and validation data, and precompute the expectation $Q_{i'j'}$ for each $(i', j')$ pair.}
